# Supplementary material for: Any6D: Model-free 6D Pose Estimation of Novel Objects
Source: arXiv:2503.18673 source file (2025-03-25)
Supplement: Supplementary file 1 [file X_suppl.tex]

\clearpage

\setcounter{page}{1}
\maketitlesupplementary

\section{Real-World Experiments}
We validate our approach by conducting experiments in real-world robot manipulation.
